# Supplementary material for: An Image-based Typology for Visualization
Source: arXiv:2403.05594 source file (2025-01-06)
Supplement: Supplementary file 1 [file supplementDatasetDrivenEvaluation.tex]

\section{\jctg{From Point-based Evaluation to Dataset Scale Evaluation}}

\noindent

Categorization is meant to be broad, as the images only need to share their essential stimuli of the coded data. A type contains both the typical items (called prototypes) and atypical ones. We focus on a meta analysis of what representations are out there in our community (Our 7.A).

Those two papers are evaluation papers. Their techniques are specific for their evaluation purpose. Our typology can help provide the evaluators a much broader set of choices – one should look at both within and cross-category plots when choosing the charts.

For example, the first paper (Xiong et al.) could have evaluated more suitable forms of visual representations for the decision tasks (whether or not to use skin creams or carry handguns in public). The tasks require an integrated display. Bars are generally good for point reading, but unsuitable for integrating between bars for rate changes. A better statistical chart is thus not to evaluate bars, but to use more visually salient line graphs or donut charts instead. See our redraw of data in Figure 1.  Thus, the conclusion would not be generalized to “Table is better”. Lines would be better at revealing patterns. 

Another bar form, donut chart may facilitate this integrated display since the arc could be more accurate for making part/whole judgments, than the arc length itself in bars.  

In this regard, our typology certainly does not have the design principle of integrated display, as we have described here. But one may use our typology to look up more suitable forms of design. Even better, instead of point evaluations, use dataset scale evaluation instead. Our community may use our typology to summarize principles between and within categories for education uses of ones’ visual literacy.

The second paper (Newburger et al.) evaluated four charts that can be conveniently mapped to our typology. 
Bar histogram -> area-based (our code)
Dot plot -> point-based
Boxplot -> bar-based and point-based
Strip plot -> bar-based 

So to evaluate these, we could potentially educate the viewers that these charts used very different essential stimuli and our typology can teach observers what information to be extracted, from these specific techniques. One may also consider if the outcomes would be reusable for techniques sharing the essential stimuli. 

We have added these two specific papers as case studies to turn point-based design to data-set based evaluation. We have also added the second paper to describe potentially generalizable design guidelines. We have credited this reviewer in our writing.
